# Supplementary material for: Impact of electromagnetic fields and heat on spin transport signals in Y$_{3}$Fe$_{5}$O$_{12}$
Source: arXiv:1906.05631 ancillary file (2019-11-06)
Supplement: Supplementary file 1 [file supporting.pdf]

# Supporting Information
## Impact of electromagnetic fields and heat on spin transport signals in $Y_3Fe_5O_{12}$

Joel Cramer,[1,2] Lorenzo Baldrati,[1] Andrew Ross,[1,2]
Mehran Vafaee,[1] Romain Lebrun,[1] and Mathias Kläui[1,2,*]

[1]*Institute of Physics, Johannes Gutenberg-University Mainz, 55099 Mainz, Germany*
[2]*Graduate School Materials Science in Mainz, 55128 Mainz, Germany*

## I. FINITE ELEMENT SIMULATION OF OERSTED FIELD DISTRIBUTION

Figure S1 shows the result of a finite element simulation regarding the spatial variation of the Oersted field that is generated when applying a charge current to the Cu wire in the non-local device described in the main text. The simulation was performed by means of the freely accessible software Agros2D[1]. In the simulation, a current density of $2 \times 10^{11}\,\mathrm{A\,m^{-2}}$ was implemented, which corresponds to a charge current of $1\,\mathrm{mA}$ applied to the Cu wire. The plot exclusively shows the $x$-component of the Oersted field.

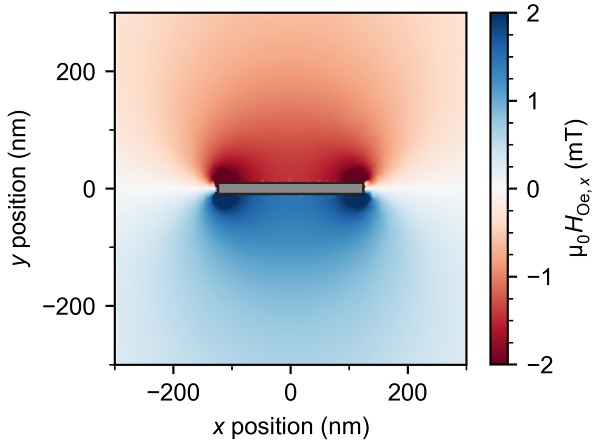


Figure S1. Spatial variation of the $x$-component of the Oersted field created by a charge current $J_{\mathrm{mid}} = 1\,\mathrm{mA}$ applied to the Cu wire and flowing into the drawing plane.

## II. MAGNETIC PROPERTIES OF YIG FILM USED

To characterize the magnetic properties of the YIG film used in this study, thermally generated voltage hysteresis loops have been recorded. In Fig. S2 the non-local spin Seebeck signal is shown, which was obtained for $\alpha = 0°$ (external field perpendicular to Pt stripes) and for different currents applied to the Cu center wire. Since the signal reflects the in-plane magnetization of the YIG[2], the voltage switching fields $H_c^{\pm} \simeq \pm 10\,\mathrm{Oe}$ correspond to the coercive fields $H_c^{\pm}$ of the YIG layer. In the main text, results obtained at low external fields ($H = \pm 50\,\mathrm{Oe}$) are discussed, at which the YIG magnetization is fully aligned along the field direction.

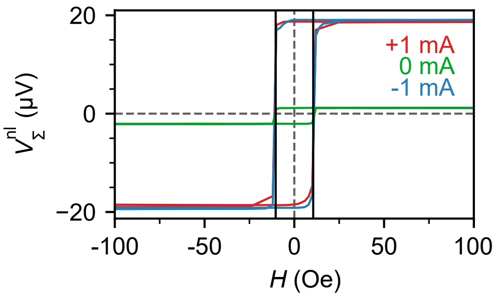


Figure S2. Hysteresis loop of non-local spin Seebeck voltage $V_{\Sigma}^{\mathrm{nl}}$ for $\alpha = 0°$ and different currents (0, $\pm 1\,\mathrm{mA}$) applied to the Cu manipulator. The black vertical lines mark the coercive field values of the YIG film.

## III. DEFINITION OF FIT FUNCTION

In the main text, a modified function is fitted to the measurement data in Fig. 3b, which shows the difference voltage signal $V_\Delta^{\mathrm{nl}}$ for the Cu $\rightarrow$ Pt configuration. Using a simplified model, this fit function reconstructs the difference between the normalized $x$-components of the YIG magnetization, which in turn is proportional to the effective field $\tilde{H}_{\mathrm{eff}}^x = H_{\mathrm{eff}}^x / H_{\mathrm{eff}}$. As the external field is known during the measurement, $H_{\mathrm{Oe}}$ serves as a fit parameter. $\tilde{H}_{\mathrm{eff}}^x(\alpha)$ is finally multiplied by a proportionality factor (plotted in Fig. 3d in the main text). The Oersted field thus determines the shape of the angular-dependent signal and for $J_{\mathrm{Cu}} = 1\,\mathrm{mA}$ (Fig. 3b main text), a value of $(27 \pm 1)\,\mathrm{Oe}$ is extracted. This value is of the same order of magnitude as the one observed in the finite element simulations. However, for such a large Oersted field and an external field of $50\,\mathrm{Oe}$, an angular shift of $\delta\alpha \approx \pm 28°$ is calculated at $\alpha = 90°$. Reconsidering the conventional non-local SSE signal $V_\Sigma^{\mathrm{nl}}$ shown in Fig. 3d in the main text, one would thus expect an amplitude of $V_\Delta^{\mathrm{nl}}$ of several µV instead of a few hundred nV, which complies better with a significantly smaller angular shift of $\delta\alpha \approx \pm 0.6°$. Eventually, this deviation is due to the fact that the Oersted field effect is restricted to a limited sample volume as compared to that which provides the non-local SSE captured by $V_\Sigma^{\mathrm{nl}}$.

* Klaeui@uni-mainz.de

[1] P. Karban, F. Mach, P. Kůs, D. Pánek, and I. Dolezel, Computing **95**, 381 (2013).
[2] A. Kehlberger, G. Jakob, M. Onbasli, D. H. Kim, C. Ross, and M. Kläui, Journal of Applied Physics **115**, 17C731 (2014).
